# Supplementary material for: Embroid: Unsupervised Prediction Smoothing Can Improve Few-Shot Classification
Source: arXiv:2307.11031 source file (2023-07-20)
Supplement: Supplementary file 1 [file bloom_multi_prompt_all.tex]

\begin{xltabular}{0.75\linewidth}{Xcccc}
\caption{\name performance for Bloom-7.1b in the multi-prompt regime (F1). Standard deviation across three prompts reported in parentheses.} \label{tab:bloom_multi_prompt_all} \\

Task    & Majority Vote & Liger & Flying Squid & \name   \\ \toprule
\endfirsthead

 Task    & Majority Vote & Liger & Flying Squid & \name   \\   \\ \toprule
\endhead

%\hline \multicolumn{3}{|r|}{{Continued on next page}} \\ \hline
\endfoot
Civil Comments& \underline{0.49}& 0.49& \underline{0.49}& 0.49\\ \midrule
Youtube& 0.80& 0.78& 0.86& \underline{0.90}\\ \midrule
World (AG News)& 0.54& 0.55& 0.54& \underline{0.58}\\ \midrule
Sports (AG News)& 0.55& 0.54& 0.55& \underline{0.63}\\ \midrule
Business (AG News)& 0.47& \underline{0.47}& 0.47& 0.47\\ \midrule
Technology (AG News)& 0.51& 0.53& 0.51& \underline{0.55}\\ \midrule
Educational Institution (DBPedia)& 0.59& 0.62& 0.60& \underline{0.67}\\ \midrule
Mean Of Transportation (DBPedia)& 0.46& \underline{0.49}& 0.46& 0.44\\ \midrule
Natural Place (DBPedia)& \underline{0.41}& 0.33& 0.33& 0.33\\ \midrule
Plant (DBPedia)& 0.81& 0.81& 0.81& \underline{0.94}\\ \midrule
Film (DBPedia)& 0.65& 0.63& 0.65& \underline{0.71}\\ \midrule
Written Work (DBPedia)& \underline{0.68}& 0.63& 0.64& 0.66\\ \midrule
Album (DBPedia)& 0.72& 0.69& 0.75& \underline{0.82}\\ \midrule
Village (DBPedia)& 0.42& 0.41& 0.41& \underline{0.44}\\ \midrule
Building (DBPedia)& 0.54& 0.55& 0.54& \underline{0.60}\\ \midrule
Company (DBPedia)& 0.63& 0.62& 0.61& \underline{0.64}\\ \midrule
Animal (DBPedia)& 0.44& \underline{0.47}& 0.44& 0.44\\ \midrule
Artist (DBPedia)& 0.56& 0.52& 0.57& \underline{0.61}\\ \midrule
Office Holder (DBPedia)& 0.64& 0.66& 0.65& \underline{0.77}\\ \midrule
Athlete (DBPedia)& \underline{0.49}& 0.47& 0.47& 0.47\\ \midrule
Part of (ChemProt)& 0.63& 0.56& 0.63& \underline{0.70}\\ \midrule
Regulator (ChemProt)& 0.51& 0.54& \underline{0.55}& 0.55\\ \midrule
Upregulator (ChemProt)& 0.52& 0.52& 0.52& \underline{0.52}\\ \midrule
Downregulator (ChemProt)& 0.53& \underline{0.54}& 0.53& 0.54\\ \midrule
Agonist (ChemProt)& 0.64& \underline{0.66}& 0.59& 0.65\\ \midrule
Antagonist (ChemProt)& 0.57& 0.58& 0.57& \underline{0.59}\\ \midrule
Substrate (ChemProt)& 0.53& 0.53& 0.53& \underline{0.53}\\ \midrule
Background (RCT)& 0.72& 0.71& 0.73& \underline{0.82}\\ \midrule
Objective (RCT)& 0.64& 0.59& 0.65& \underline{0.65}\\ \midrule
Methods (RCT)& 0.63& 0.58& 0.58& \underline{0.63}\\ \midrule
Results (RCT)& 0.37& \underline{0.47}& 0.37& 0.33\\ \midrule
Conclusions (RCT)& \underline{0.37}& 0.35& 0.34& 0.33\\ \midrule
Affiliate License-Licensee (CUAD)& \underline{0.66}& \underline{0.66}& \underline{0.66}& 0.66\\ \midrule
Anti-Assignment (CUAD)& 0.69& 0.71& 0.70& \underline{0.80}\\ \midrule
Audit Rights (CUAD)& 0.67& 0.69& 0.62& \underline{0.69}\\ \midrule
Cap On Liability (CUAD)& 0.67& 0.67& 0.67& \underline{0.72}\\ \midrule
Change Of Control (CUAD)& 0.51& \underline{0.56}& 0.48& 0.50\\ \midrule
Competitive Restriction Exception (CUAD)& 0.57& 0.58& 0.57& \underline{0.60}\\ \midrule
Covenant Not To Sue (CUAD)& 0.52& \underline{0.60}& 0.51& 0.54\\ \midrule
Exclusivity (CUAD)& 0.51& 0.51& 0.51& \underline{0.54}\\ \midrule
Insurance (CUAD)& 0.71& 0.71& 0.71& \underline{0.76}\\ \midrule
Ip Ownership Assignment (CUAD)& 0.65& 0.67& 0.67& \underline{0.68}\\ \midrule
Irrevocable Or Perpetual License (CUAD)& 0.82& 0.83& 0.82& \underline{0.87}\\ \midrule
Joint Ip Ownership (CUAD)& 0.69& 0.73& \underline{0.74}& 0.74\\ \midrule
License Grant (CUAD)& 0.77& 0.75& 0.78& \underline{0.82}\\ \midrule
Liquidated Damages (CUAD)& 0.72& 0.76& 0.72& \underline{0.83}\\ \midrule
Minimum Commitment (CUAD)& 0.53& 0.53& 0.53& \underline{0.55}\\ \midrule
No-Solicit Of Employees (CUAD)& 0.72& 0.72& 0.72& \underline{0.85}\\ \midrule
Non-Compete (CUAD)& 0.60& 0.60& 0.58& \underline{0.62}\\ \midrule
Non-Disparagement (CUAD)& 0.64& 0.62& 0.64& \underline{0.65}\\ \midrule
Non-Transferable License (CUAD)& 0.74& 0.73& 0.74& \underline{0.76}\\ \midrule
Post-Termination Services (CUAD)& \underline{0.57}& 0.56& \underline{0.57}& 0.57\\ \midrule
Revenue-Profit Sharing (CUAD)& 0.74& 0.75& 0.74& \underline{0.79}\\ \midrule
Rofr-Rofo-Rofn (CUAD)& \underline{0.51}& \underline{0.51}& \underline{0.51}& 0.50\\ \midrule
Source Code Escrow (CUAD)& \underline{0.75}& 0.73& \underline{0.75}& 0.74\\ \midrule
Termination For Convenience (CUAD)& 0.55& 0.59& \underline{0.69}& 0.68\\ \midrule
Uncapped Liability (CUAD)& 0.68& 0.67& 0.68& \underline{0.82}\\ \midrule
Volume Restriction (CUAD)& \underline{0.56}& 0.56& \underline{0.56}& 0.54\\ \midrule
Effective Date (CUAD)& 0.51& 0.51& 0.51& \underline{0.56}\\ \midrule
Renewal Term (CUAD)& 0.90& 0.89& 0.90& \underline{0.94}\\ \midrule
Expiration Date (CUAD)& 0.71& 0.71& 0.71& \underline{0.79}\\ \midrule
Governing Law (CUAD)& 0.55& 0.57& 0.53& \underline{0.58}\\ \midrule
Warranty Duration (CUAD)& 0.76& 0.76& 0.75& \underline{0.81}\\ \midrule
Notice Period To Terminate Renewal (CUAD)& 0.87& 0.86& 0.90& \underline{0.91}\\ \midrule
HE (Learned Hands)& \underline{0.70}& 0.68& 0.65& 0.69\\ \midrule
MO (Learned Hands)& \underline{0.58}& 0.57& 0.57& 0.57\\ \midrule
CR (Learned Hands)& \underline{0.65}& 0.65& 0.65& 0.63\\ \midrule
CO (Learned Hands)& \underline{0.72}& 0.71& 0.64& 0.69\\ \midrule
HO (Learned Hands)& 0.71& 0.69& 0.65& \underline{0.78}\\ \midrule
BU (Learned Hands)& 0.73& 0.73& 0.72& \underline{0.79}\\ \midrule
TO (Learned Hands)& \underline{0.60}& 0.57& 0.57& 0.52\\ \midrule
TR (Learned Hands)& 0.50& \underline{0.51}& 0.48& 0.36\\ \midrule
WO (Learned Hands)& 0.61& 0.62& 0.61& \underline{0.67}\\ \midrule
ES (Learned Hands)& 0.79& 0.82& 0.85& \underline{0.89}\\ \midrule
FA (Learned Hands)& 0.70& 0.71& 0.70& \underline{0.73}\\ \midrule
Architect (FewRel)& 0.91& 0.89& 0.91& \underline{0.96}\\ \midrule
Composer (FewRel)& 0.84& 0.83& 0.85& \underline{0.92}\\ \midrule
Country (FewRel)& 0.58& 0.61& 0.59& \underline{0.63}\\ \midrule
Developer (FewRel)& 0.86& 0.84& 0.86& \underline{0.94}\\ \midrule
Director (FewRel)& 0.86& 0.84& 0.86& \underline{0.90}\\ \midrule
Distributor (FewRel)& 0.85& 0.84& 0.85& \underline{0.89}\\ \midrule
Father (FewRel)& 0.76& 0.74& 0.74& \underline{0.87}\\ \midrule
Instrument (FewRel)& 0.90& 0.89& 0.93& \underline{0.93}\\ \midrule
League (FewRel)& 0.83& 0.82& 0.83& \underline{0.92}\\ \midrule
Platform (FewRel)& 0.81& 0.77& 0.82& \underline{0.89}\\ \midrule
Participating Team (FewRel)& 0.90& 0.76& 0.90& \underline{0.96}\\ \midrule
Military Branch (FewRel)& 0.86& 0.82& 0.86& \underline{0.93}\\ \midrule
Movement (FewRel)& 0.80& 0.79& 0.80& \underline{0.88}\\ \midrule
Sibling (FewRel)& 0.78& 0.78& 0.78& \underline{0.90}\\ \midrule
Successful Candidate (FewRel)& 0.82& 0.82& 0.82& \underline{0.93}\\ \midrule
Taxon Rank (FewRel)& 0.96& 0.97& 0.98& \underline{0.99}\\ \midrule
Tributary (FewRel)& 0.83& 0.81& 0.83& \underline{0.94}\\ \midrule
Occupation (FewRel)& 0.76& 0.76& 0.76& \underline{0.78}\\ \midrule
Winner (FewRel)& 0.80& 0.82& 0.80& \underline{0.85}\\ \midrule
Genre (FewRel)& 0.75& 0.70& 0.75& \underline{0.80}\\ 
\bottomrule
\endlastfoot 
\end{xltabular}
