# Supplementary material for: Embroid: Unsupervised Prediction Smoothing Can Improve Few-Shot Classification
Source: arXiv:2307.11031 source file (2023-07-20)
Supplement: Supplementary file 3 [file opt_multi_prompt_all.tex]

\newpage
\begin{xltabular}{0.75\linewidth}{Xcccc}
\caption{\name performance for OPT-6.7B in the multi-prompt regime (F1). Standard deviation across three prompts reported in parentheses.} \label{tab:opt_multi_prompt_all} \\
 Task    & Majority Vote & Liger & Flying Squid & \name   \\   \\ \toprule
\endhead
%\hline \multicolumn{3}{|r|}{{Continued on next page}} \\ \hline
\endfoot
Civil Comments& \underline{0.48}& 0.47& 0.47& 0.47\\ \midrule
Youtube& 0.81& 0.85& 0.83& \underline{0.88}\\ \midrule
World (AG News)& 0.53& \underline{0.55}& 0.54& 0.52\\ \midrule
Sports (AG News)& 0.69& 0.62& 0.69& \underline{0.82}\\ \midrule
Business (AG News)& \underline{0.51}& 0.51& \underline{0.51}& 0.50\\ \midrule
Technology (AG News)& 0.60& 0.59& 0.58& \underline{0.67}\\ \midrule
Educational Institution (DBPedia)& 0.60& 0.62& 0.53& \underline{0.63}\\ \midrule
Mean Of Transportation (DBPedia)& 0.50& 0.50& 0.49& \underline{0.52}\\ \midrule
Natural Place (DBPedia)& 0.78& 0.80& 0.79& \underline{0.86}\\ \midrule
Plant (DBPedia)& 0.73& 0.66& 0.73& \underline{0.81}\\ \midrule
Film (DBPedia)& 0.57& 0.58& \underline{0.63}& 0.62\\ \midrule
Album (DBPedia)& 0.75& 0.64& 0.75& \underline{0.93}\\ \midrule
Village (DBPedia)& 0.61& 0.60& 0.60& \underline{0.64}\\ \midrule
Building (DBPedia)& 0.65& 0.62& 0.64& \underline{0.73}\\ \midrule
Company (DBPedia)& \underline{0.49}& 0.46& 0.49& 0.40\\ \midrule
Animal (DBPedia)& 0.69& 0.67& 0.69& \underline{0.79}\\ \midrule
Artist (DBPedia)& 0.70& 0.69& 0.70& \underline{0.82}\\ \midrule
Office Holder (DBPedia)& 0.59& 0.58& 0.59& \underline{0.63}\\ \midrule
Athlete (DBPedia)& 0.51& \underline{0.52}& 0.52& 0.52\\ \midrule
Part of (ChemProt)& 0.46& \underline{0.49}& 0.45& 0.34\\ \midrule
Regulator (ChemProt)& 0.53& 0.51& \underline{0.53}& 0.52\\ \midrule
Upregulator (ChemProt)& 0.65& 0.61& 0.65& \underline{0.71}\\ \midrule
Downregulator (ChemProt)& \underline{0.48}& 0.48& \underline{0.48}& 0.40\\ \midrule
Agonist (ChemProt)& 0.51& \underline{0.51}& 0.51& 0.48\\ \midrule
Antagonist (ChemProt)& \underline{0.48}& 0.48& \underline{0.48}& 0.40\\ \midrule
Substrate (ChemProt)& 0.54& 0.53& 0.54& \underline{0.56}\\ \midrule
Background (RCT)& 0.44& \underline{0.45}& 0.44& 0.43\\ \midrule
Objective (RCT)& 0.67& 0.66& 0.66& \underline{0.72}\\ \midrule
Methods (RCT)& 0.56& 0.58& 0.44& \underline{0.60}\\ \midrule
Results (RCT)& 0.59& 0.60& 0.59& \underline{0.61}\\ \midrule
Conclusions (RCT)& 0.61& 0.58& 0.61& \underline{0.67}\\ \midrule
Affiliate License-Licensee (CUAD)& \underline{0.69}& 0.68& \underline{0.69}& 0.63\\ \midrule
Anti-Assignment (CUAD)& 0.40& \underline{0.46}& 0.40& 0.37\\ \midrule
Audit Rights (CUAD)& 0.68& 0.65& 0.64& \underline{0.72}\\ \midrule
Cap On Liability (CUAD)& 0.51& 0.51& 0.51& \underline{0.57}\\ \midrule
Change Of Control (CUAD)& 0.57& 0.57& \underline{0.63}& 0.49\\ \midrule
Competitive Restriction Exception (CUAD)& \underline{0.39}& 0.38& 0.35& 0.34\\ \midrule
Covenant Not To Sue (CUAD)& \underline{0.47}& 0.46& 0.45& 0.47\\ \midrule
Exclusivity (CUAD)& 0.60& 0.60& 0.60& \underline{0.61}\\ \midrule
Insurance (CUAD)& 0.65& 0.63& 0.61& \underline{0.68}\\ \midrule
Ip Ownership Assignment (CUAD)& 0.71& 0.71& 0.71& \underline{0.74}\\ \midrule
Irrevocable Or Perpetual License (CUAD)& 0.79& 0.81& 0.79& \underline{0.85}\\ \midrule
Joint Ip Ownership (CUAD)& 0.68& 0.68& 0.68& \underline{0.70}\\ \midrule
License Grant (CUAD)& 0.76& 0.76& 0.77& \underline{0.83}\\ \midrule
Liquidated Damages (CUAD)& \underline{0.46}& 0.42& \underline{0.46}& 0.40\\ \midrule
Minimum Commitment (CUAD)& \underline{0.55}& 0.48& 0.46& 0.48\\ \midrule
No-Solicit Of Employees (CUAD)& 0.73& 0.73& 0.73& \underline{0.79}\\ \midrule
Non-Compete (CUAD)& \underline{0.41}& 0.39& 0.30& 0.36\\ \midrule
Non-Disparagement (CUAD)& 0.39& \underline{0.50}& 0.35& 0.35\\ \midrule
Non-Transferable License (CUAD)& 0.62& 0.63& 0.69& \underline{0.72}\\ \midrule
Post-Termination Services (CUAD)& \underline{0.57}& \underline{0.57}& \underline{0.57}& 0.56\\ \midrule
Revenue-Profit Sharing (CUAD)& 0.64& 0.63& 0.64& \underline{0.74}\\ \midrule
Rofr-Rofo-Rofn (CUAD)& 0.54& 0.55& 0.55& \underline{0.56}\\ \midrule
Source Code Escrow (CUAD)& 0.65& 0.63& 0.62& \underline{0.69}\\ \midrule
Termination For Convenience (CUAD)& 0.78& 0.78& 0.78& \underline{0.79}\\ \midrule
Uncapped Liability (CUAD)& 0.49& 0.50& 0.50& \underline{0.59}\\ \midrule
Volume Restriction (CUAD)& 0.54& 0.54& 0.54& \underline{0.55}\\ \midrule
Effective Date (CUAD)& 0.92& 0.91& 0.92& \underline{0.93}\\ \midrule
Renewal Term (CUAD)& 0.79& 0.75& 0.78& \underline{0.87}\\ \midrule
Expiration Date (CUAD)& 0.74& 0.74& 0.74& \underline{0.87}\\ \midrule
Governing Law (CUAD)& 0.88& 0.84& 0.89& \underline{0.94}\\ \midrule
Warranty Duration (CUAD)& 0.54& 0.54& 0.54& \underline{0.57}\\ \midrule
Notice Period To Terminate Renewal (CUAD)& 0.81& 0.78& 0.81& \underline{0.85}\\ \midrule
HE (Learned Hands)& 0.74& 0.75& \underline{0.79}& 0.77\\ \midrule
MO (Learned Hands)& \underline{0.57}& 0.54& 0.55& 0.54\\ \midrule
CR (Learned Hands)& 0.73& 0.72& 0.71& \underline{0.74}\\ \midrule
CO (Learned Hands)& 0.62& 0.61& \underline{0.67}& 0.62\\ \midrule
HO (Learned Hands)& 0.83& 0.83& 0.83& \underline{0.86}\\ \midrule
BU (Learned Hands)& 0.75& 0.69& 0.75& \underline{0.78}\\ \midrule
TO (Learned Hands)& 0.62& 0.55& 0.62& \underline{0.62}\\ \midrule
TR (Learned Hands)& 0.71& 0.71& 0.71& \underline{0.77}\\ \midrule
WO (Learned Hands)& 0.78& 0.78& 0.78& \underline{0.83}\\ \midrule
ES (Learned Hands)& 0.82& 0.85& 0.82& \underline{0.87}\\ \midrule
FA (Learned Hands)& 0.69& 0.68& 0.69& \underline{0.72}\\ \midrule
Architect (FewRel)& 0.83& 0.77& 0.83& \underline{0.94}\\ \midrule
Composer (FewRel)& 0.85& 0.86& 0.85& \underline{0.89}\\ \midrule
Country (FewRel)& 0.61& 0.61& 0.61& \underline{0.65}\\ \midrule
Developer (FewRel)& 0.83& 0.83& 0.83& \underline{0.93}\\ \midrule
Director (FewRel)& 0.84& 0.86& 0.85& \underline{0.88}\\ \midrule
Distributor (FewRel)& 0.80& 0.80& 0.80& \underline{0.88}\\ \midrule
Father (FewRel)& 0.76& 0.76& 0.76& \underline{0.91}\\ \midrule
Instrument (FewRel)& 0.86& 0.87& 0.87& \underline{0.96}\\ \midrule
League (FewRel)& 0.83& 0.76& 0.83& \underline{0.92}\\ \midrule
Platform (FewRel)& 0.73& 0.70& 0.73& \underline{0.85}\\ \midrule
Participating Team (FewRel)& 0.80& 0.74& 0.80& \underline{0.93}\\ \midrule
Military Branch (FewRel)& 0.83& 0.80& 0.83& \underline{0.94}\\ \midrule
Movement (FewRel)& 0.80& 0.78& 0.80& \underline{0.90}\\ \midrule
Sibling (FewRel)& 0.82& 0.83& 0.82& \underline{0.90}\\ \midrule
Successful Candidate (FewRel)& 0.88& 0.87& 0.88& \underline{0.97}\\ \midrule
Taxon Rank (FewRel)& 0.83& 0.85& 0.84& \underline{0.97}\\ \midrule
Tributary (FewRel)& 0.90& 0.90& 0.90& \underline{0.97}\\ \midrule
Occupation (FewRel)& 0.54& 0.54& \underline{0.55}& 0.55\\ \midrule
Winner (FewRel)& 0.69& 0.68& 0.69& \underline{0.77}\\ \midrule
Genre (FewRel)& 0.71& 0.66& 0.71& \underline{0.77}\\
\bottomrule
\endlastfoot 
\end{xltabular}
