# Supplementary material for: Embroid: Unsupervised Prediction Smoothing Can Improve Few-Shot Classification
Source: arXiv:2307.11031 source file (2023-07-20)
Supplement: Supplementary file 4 [file single_prompt_all_results.tex]

\begin{xltabular}{\textwidth}{Xcccccc}
\caption{\name performance in single-prompt regime (F1). Standard deviation across three prompts reported in parentheses.} \label{tab:single_prompt_all_tasks} \\

 &\multicolumn{2}{c}{GPT-JT-6b} & \multicolumn{2}{c}{Bloom-7b1} & \multicolumn{2}{c}{OPT-6.7b} \\ \cmidrule(lr){2-7}
      Task    & Base Prompt & \name & Base Prompt & \name & Base Prompt & \name  \\ \toprule
\endfirsthead

 &\multicolumn{2}{c}{GPT-JT-6b} &\multicolumn{2}{c}{Bloom-7b1} & \multicolumn{2}{c}{OPT-6.7b} \\ \cmidrule(lr){2-7}
      Task    & Base Prompt & \name & Base Prompt & \name & Base Prompt & \name  \\ \toprule
\endhead

%\hline \multicolumn{3}{|r|}{{Continued on next page}} \\ \hline
\endfoot

\bottomrule
\endlastfoot 
Civil Comments& \underline{0.49} (0.01) & 0.47 (0.00)& 0.49 (0.01)& \underline{0.49} (0.02)& \underline{0.52} (0.01) & 0.47 (0.00)\\ \midrule
Youtube& 0.71 (0.04)& \underline{0.72} (0.05)& 0.76 (0.10)& \underline{0.81} (0.12)& 0.74 (0.01)& \underline{0.78} (0.03)\\ \midrule
World (AG News)& 0.70 (0.05)& \underline{0.76} (0.13)& 0.53 (0.04)& \underline{0.55} (0.11)& \underline{0.52} (0.01) & 0.49 (0.06)\\ \midrule
Sports (AG News)& 0.59 (0.02)& \underline{0.61} (0.12)& 0.55 (0.01)& \underline{0.63} (0.01)& 0.67 (0.02)& \underline{0.78} (0.08)\\ \midrule
Business (AG News)& 0.57 (0.05)& \underline{0.61} (0.13)& \underline{0.47} (0.01) & 0.46 (0.03)& 0.51 (0.01)& \underline{0.52} (0.04)\\ \midrule
Technology (AG News)& 0.64 (0.05)& \underline{0.65} (0.11)& 0.52 (0.01)& \underline{0.55} (0.02)& 0.57 (0.01)& \underline{0.64} (0.02)\\ \midrule
Educational Institution (DBPedia)& 0.75 (0.04)& \underline{0.84} (0.06)& 0.58 (0.03)& \underline{0.62} (0.08)& \underline{0.56} (0.02) & 0.52 (0.06)\\ \midrule
Mean Of Transportation (DBPedia)& 0.63 (0.04)& \underline{0.68} (0.06)& \underline{0.47} (0.03) & 0.45 (0.03)& \underline{0.49} (0.04) & 0.49 (0.07)\\ \midrule
Natural Place (DBPedia)& 0.73 (0.01)& \underline{0.80} (0.02)& \underline{0.46} (0.06) & 0.46 (0.12)& 0.73 (0.06)& \underline{0.79} (0.06)\\ \midrule
Plant (DBPedia)& 0.71 (0.05)& \underline{0.80} (0.09)& 0.80 (0.09)& \underline{0.88} (0.06)& 0.72 (0.00)& \underline{0.80} (0.02)\\ \midrule
Film (DBPedia)& 0.74 (0.02)& \underline{0.81} (0.01)& 0.64 (0.05)& \underline{0.66} (0.09)& \underline{0.57} (0.08) & 0.56 (0.19)\\ \midrule
Written Work (DBPedia)& 0.65 (0.03)& \underline{0.71} (0.05)& 0.66 (0.04)& \underline{0.68} (0.06)& \underline{0.40} (0) & 0.33 (0)\\ \midrule
Album (DBPedia)& 0.79 (0.03)& \underline{0.92} (0.05)& 0.70 (0.05)& \underline{0.78} (0.07)& 0.74 (0.11)& \underline{0.86} (0.11)\\ \midrule
Village (DBPedia)& 0.80 (0.02)& \underline{0.89} (0.04)& 0.42 (0.08)& \underline{0.44} (0.10)& 0.57 (0.08)& \underline{0.59} (0.10)\\ \midrule
Building (DBPedia)& 0.75 (0.01)& \underline{0.87} (0.02)& 0.54 (0.00)& \underline{0.57} (0.02)& 0.66 (0.04)& \underline{0.73} (0.04)\\ \midrule
Company (DBPedia)& 0.72 (0.02)& \underline{0.77} (0.03)& 0.59 (0.05)& \underline{0.60} (0.09)& \underline{0.46} (0.03) & 0.42 (0.03)\\ \midrule
Animal (DBPedia)& 0.71 (0.01)& \underline{0.79} (0.03)& 0.45 (0.03)& \underline{0.46} (0.04)& 0.68 (0.08)& \underline{0.75} (0.12)\\ \midrule
Artist (DBPedia)& 0.79 (0.01)& \underline{0.87} (0.01)& 0.55 (0.02)& \underline{0.59} (0.03)& 0.68 (0.02)& \underline{0.76} (0.09)\\ \midrule
Office Holder (DBPedia)& 0.83 (0.05)& \underline{0.91} (0.02)& 0.63 (0.02)& \underline{0.71} (0.06)& 0.58 (0.03)& \underline{0.60} (0.04)\\ \midrule
Athlete (DBPedia)& 0.83 (0.02)& \underline{0.90} (0.01)& 0.48 (0.02)& \underline{0.48} (0.03)& \underline{0.49} (0.03) & 0.48 (0.08)\\ \midrule
Part Of (ChemProt)& 0.64 (0.06)& \underline{0.69} (0.09)& 0.61 (0.07)& \underline{0.66} (0.07)& 0.50 (0.02)& \underline{0.53} (0.04)\\ \midrule
Regulator (ChemProt)& \underline{0.50} (0.01) & 0.49 (0.01)& \underline{0.52} (0.02) & 0.52 (0.05)& 0.50 (0.03)& \underline{0.51} (0.03)\\ \midrule
Upregulator (ChemProt)& 0.63 (0.01)& \underline{0.66} (0.02)& \underline{0.52} (0.01) & 0.51 (0.02)& 0.63 (0.01)& \underline{0.67} (0.02)\\ \midrule
Downregulator (ChemProt)& 0.57 (0.01)& \underline{0.58} (0.02)& \underline{0.51} (0.01) & 0.51 (0.02)& 0.52 (0.01)& \underline{0.54} (0.02)\\ \midrule
Agonist (ChemProt)& \underline{0.61} (0.02) & 0.59 (0.09)& \underline{0.60} (0.02) & 0.59 (0.06)& \underline{0.52} (0.01) & 0.50 (0.08)\\ \midrule
Antagonist (ChemProt)& 0.58 (0.04)& \underline{0.60} (0.05)& 0.56 (0.00)& \underline{0.57} (0.01)& \underline{0.48} (0.01) & 0.46 (0.05)\\ \midrule
Substrate (ChemProt)& 0.63 (0.01)& \underline{0.66} (0.01)& 0.52 (0.01)& \underline{0.53} (0.01)& 0.54 (0.01)& \underline{0.55} (0.03)\\ \midrule
Background (RCT)& 0.61 (0.04)& \underline{0.64} (0.06)& 0.69 (0.01)& \underline{0.75} (0.02)& \underline{0.44} (0.01) & 0.43 (0.03)\\ \midrule
Objective (RCT)& 0.73 (0.01)& \underline{0.81} (0.04)& 0.61 (0.01)& \underline{0.64} (0.00)& 0.62 (0.02)& \underline{0.68} (0.03)\\ \midrule
Methods (RCT)& 0.69 (0.03)& \underline{0.75} (0.09)& 0.60 (0.04)& \underline{0.64} (0.11)& 0.51 (0.05)& \underline{0.54} (0.07)\\ \midrule
Results (RCT)& 0.60 (0.04)& \underline{0.63} (0.06)& \underline{0.44} (0.02) & 0.41 (0.02)& 0.56 (0.03)& \underline{0.60} (0.03)\\ \midrule
Conclusions (RCT)& 0.65 (0.02)& \underline{0.73} (0.02)& \underline{0.47} (0.00) & 0.46 (0.03)& 0.60 (0.00)& \underline{0.66} (0.01)\\ \midrule
Affiliate License-Licensee (CUAD)& \underline{0.86} (0.03) & 0.86 (0.02)& \underline{0.67} (0.02) & 0.67 (0.03)& \underline{0.63} (0.08) & 0.57 (0.14)\\ \midrule
Anti-Assignment (CUAD)& 0.79 (0.03)& \underline{0.84} (0.01)& 0.65 (0.14)& \underline{0.67} (0.15)& \underline{0.41} (0.02) & 0.38 (0.07)\\ \midrule
Audit Rights (CUAD)& 0.84 (0.02)& \underline{0.89} (0.03)& \underline{0.61} (0.01) & 0.60 (0.02)& 0.65 (0.04)& \underline{0.65} (0.07)\\ \midrule
Cap On Liability (CUAD)& 0.78 (0.06)& \underline{0.82} (0.05)& 0.64 (0.05)& \underline{0.66} (0.07)& 0.49 (0.05)& \underline{0.55} (0.10)\\ \midrule
Change Of Control (CUAD)& 0.70 (0.05)& \underline{0.71} (0.06)& 0.52 (0.08)& \underline{0.52} (0.10)& 0.57 (0.00)& \underline{0.61} (0.02)\\ \midrule
Competitive Restriction Exception (CUAD)& \underline{0.59} (0.04) & 0.58 (0.03)& \underline{0.53} (0.03) & 0.52 (0.07)& \underline{0.44} (0.05) & 0.44 (0.09)\\ \midrule
Cove0t Not To Sue (CUAD)& 0.75 (0.02)& \underline{0.75} (0.02)& 0.51 (0.18)& \underline{0.51} (0.19)& 0.47 (0.03)& \underline{0.48} (0.05)\\ \midrule
Exclusivity (CUAD)& \underline{0.72} (0.00) & 0.71 (0.01)& 0.51 (0.01)& \underline{0.51} (0.03)& 0.58 (0.02)& \underline{0.59} (0.00)\\ \midrule
Insurance (CUAD)& 0.80 (0.02)& \underline{0.86} (0.02)& 0.68 (0.07)& \underline{0.73} (0.07)& 0.62 (0.06)& \underline{0.64} (0.07)\\ \midrule
Ip Ownership Assignment (CUAD)& 0.75 (0.01)& \underline{0.76} (0.01)& \underline{0.62} (0.05) & 0.61 (0.07)& 0.68 (0.06)& \underline{0.71} (0.07)\\ \midrule
Irrevocable Or Perpetual License (CUAD)& \underline{0.87} (0.04) & 0.86 (0.01)& 0.81 (0.04)& \underline{0.84} (0.06)& \underline{0.79} (0.03) & 0.78 (0.04)\\ \midrule
Joint Ip Ownership (CUAD)& \underline{0.77} (0.03) & 0.76 (0.04)& 0.69 (0.02)& \underline{0.74} (0.07)& 0.67 (0.01)& \underline{0.68} (0.01)\\ \midrule
License Grant (CUAD)& 0.86 (0.00)& \underline{0.87} (0.01)& 0.75 (0.02)& \underline{0.77} (0.02)& 0.70 (0.09)& \underline{0.71} (0.14)\\ \midrule
Liquidated Damages (CUAD)& 0.78 (0.04)& \underline{0.79} (0.05)& 0.69 (0.01)& \underline{0.75} (0.04)& \underline{0.45} (0.02) & 0.42 (0.07)\\ \midrule
Minimum Commitment (CUAD)& 0.72 (0.03)& \underline{0.75} (0.07)& \underline{0.53} (0.00) & 0.53 (0.02)& 0.53 (0.01)& \underline{0.55} (0.03)\\ \midrule
No-Solicit Of Employees (CUAD)& 0.94 (0.01)& \underline{0.96} (0.00)& 0.74 (0.04)& \underline{0.78} (0.12)& 0.69 (0.01)& \underline{0.76} (0.04)\\ \midrule
Non-Compete (CUAD)& \underline{0.73} (0.02) & 0.73 (0.02)& \underline{0.56} (0.09) & 0.56 (0.10)& \underline{0.41} (0.04) & 0.40 (0.03)\\ \midrule
Non-Disparagement (CUAD)& 0.85 (0.04)& \underline{0.87} (0.03)& \underline{0.62} (0.03) & 0.60 (0.01)& \underline{0.50} (0.01) & 0.45 (0.09)\\ \midrule
Non-Transferable License (CUAD)& 0.82 (0.00)& \underline{0.83} (0.01)& 0.73 (0.02)& \underline{0.75} (0.01)& 0.60 (0.09)& \underline{0.63} (0.11)\\ \midrule
Post-Termination Services (CUAD)& 0.64 (0.04)& \underline{0.65} (0.04)& \underline{0.58} (0.00) & 0.56 (0.00)& \underline{0.56} (0.02) & 0.55 (0.06)\\ \midrule
Revenue-Profit Sharing (CUAD)& 0.71 (0.02)& \underline{0.74} (0.02)& 0.70 (0.03)& \underline{0.74} (0.04)& 0.65 (0.03)& \underline{0.69} (0.04)\\ \midrule
Rofr-Rofo-Rofn (CUAD)& \underline{0.64} (0.02) & 0.62 (0.06)& 0.50 (0.02)& \underline{0.51} (0.02)& \underline{0.54} (0.01) & 0.54 (0.01)\\ \midrule
Source Code Escrow (CUAD)& \underline{0.70} (0.00) & 0.69 (0.02)& 0.71 (0.05)& \underline{0.71} (0.15)& 0.60 (0.04)& \underline{0.65} (0.06)\\ \midrule
Termination For Convenience (CUAD)& 0.82 (0.01)& \underline{0.84} (0.02)& \underline{0.58} (0.10) & 0.54 (0.16)& 0.76 (0.04)& \underline{0.78} (0.01)\\ \midrule
Uncapped Liability (CUAD)& 0.86 (0.02)& \underline{0.91} (0.01)& 0.70 (0.04)& \underline{0.80} (0.01)& 0.49 (0.05)& \underline{0.58} (0.07)\\ \midrule
Volume Restriction (CUAD)& 0.66 (0.06)& \underline{0.68} (0.05)& \underline{0.54} (0.03) & 0.51 (0.04)& \underline{0.53} (0.02) & 0.52 (0.05)\\ \midrule
Effective Date (CUAD)& 0.86 (0.04)& \underline{0.88} (0.07)& 0.55 (0.08)& \underline{0.60} (0.14)& 0.86 (0.04)& \underline{0.92} (0.02)\\ \midrule
Renewal Term (CUAD)& 0.78 (0.04)& \underline{0.87} (0.03)& 0.86 (0.06)& \underline{0.90} (0.02)& 0.75 (0.05)& \underline{0.86} (0.02)\\ \midrule
Expiration Date (CUAD)& 0.86 (0.03)& \underline{0.89} (0.01)& 0.70 (0.04)& \underline{0.77} (0.05)& 0.77 (0.05)& \underline{0.85} (0.02)\\ \midrule
Governing Law (CUAD)& 0.91 (0.05)& \underline{0.97} (0.02)& 0.52 (0.00)& \underline{0.55} (0.01)& 0.86 (0.04)& \underline{0.91} (0.02)\\ \midrule
Warranty Duration (CUAD)& \underline{0.72} (0.01) & 0.72 (0.04)& \underline{0.74} (0.01) & 0.72 (0.03)& \underline{0.54} (0.01) & 0.54 (0.00)\\ \midrule
Notice Period To Terminate Renewal (CUAD)& 0.88 (0.02)& \underline{0.89} (0.01)& 0.88 (0.01)& \underline{0.88} (0.05)& 0.80 (0.03)& \underline{0.85} (0.04)\\ \midrule
HE (Learned Hands)& \underline{0.73} (0.03) & 0.73 (0.03)& \underline{0.68} (0.04) & 0.66 (0.04)& \underline{0.75} (0.04) & 0.74 (0.04)\\ \midrule
MO (Learned Hands)& 0.55 (0.01)& \underline{0.56} (0.00)& \underline{0.56} (0.02) & 0.55 (0.03)& \underline{0.54} (0.02) & 0.54 (0.03)\\ \midrule
CR (Learned Hands)& 0.74 (0.02)& \underline{0.74} (0.02)& \underline{0.59} (0.03) & 0.55 (0.12)& 0.71 (0.02)& \underline{0.72} (0.01)\\ \midrule
CO (Learned Hands)& 0.67 (0.02)& \underline{0.68} (0.01)& \underline{0.65} (0.02) & 0.62 (0.03)& 0.63 (0.02)& \underline{0.63} (0.03)\\ \midrule
HO (Learned Hands)& 0.75 (0.06)& \underline{0.77} (0.07)& 0.69 (0.11)& \underline{0.73} (0.13)& 0.83 (0.00)& \underline{0.85} (0.02)\\ \midrule
BU (Learned Hands)& \underline{0.71} (0.05) & 0.67 (0.03)& 0.72 (0.02)& \underline{0.74} (0.04)& 0.74 (0.05)& \underline{0.76} (0.05)\\ \midrule
TO (Learned Hands)& \underline{0.63} (0.03) & 0.60 (0.05)& 0.56 (0.01)& \underline{0.59} (0.02)& 0.64 (0.02)& \underline{0.65} (0.04)\\ \midrule
TR (Learned Hands)& 0.60 (0.02)& \underline{0.61} (0.03)& \underline{0.54} (0.04) & 0.50 (0.11)& 0.68 (0.05)& \underline{0.72} (0.07)\\ \midrule
WO (Learned Hands)& 0.60 (0.02)& \underline{0.63} (0.03)& \underline{0.60} (0.02) & 0.58 (0.07)& 0.76 (0.03)& \underline{0.79} (0.05)\\ \midrule
ES (Learned Hands)& \underline{0.64} (0.05) & 0.60 (0.17)& \underline{0.79} (0.03) & 0.78 (0.06)& \underline{0.78} (0.03) & 0.78 (0.03)\\ \midrule
FA (Learned Hands)& 0.65 (0.02)& \underline{0.68} (0.03)& 0.66 (0.03)& \underline{0.67} (0.02)& 0.66 (0.01)& \underline{0.68} (0.01)\\ \midrule
Architect (FewRel)& 0.87 (0.02)& \underline{0.92} (0.03)& 0.86 (0.04)& \underline{0.92} (0.06)& 0.81 (0.00)& \underline{0.90} (0.06)\\ \midrule
Composer (FewRel)& 0.85 (0.00)& \underline{0.89} (0.03)& 0.82 (0.01)& \underline{0.90} (0.01)& 0.84 (0.01)& \underline{0.88} (0.02)\\ \midrule
Country (FewRel)& 0.62 (0.04)& \underline{0.66} (0.05)& 0.60 (0.02)& \underline{0.61} (0.02)& 0.60 (0.04)& \underline{0.61} (0.12)\\ \midrule
Developer (FewRel)& 0.77 (0.01)& \underline{0.80} (0.01)& 0.85 (0.01)& \underline{0.91} (0.03)& 0.81 (0.02)& \underline{0.92} (0.01)\\ \midrule
Director (FewRel)& 0.87 (0.00)& \underline{0.89} (0.01)& 0.85 (0.05)& \underline{0.88} (0.02)& 0.84 (0.01)& \underline{0.88} (0.01)\\ \midrule
Distributor (FewRel)& 0.81 (0.01)& \underline{0.86} (0.02)& 0.83 (0.01)& \underline{0.88} (0.00)& 0.79 (0.01)& \underline{0.87} (0.01)\\ \midrule
Father (FewRel)& 0.75 (0.04)& \underline{0.82} (0.06)& 0.72 (0.02)& \underline{0.80} (0.04)& 0.76 (0.03)& \underline{0.87} (0.03)\\ \midrule
Instrument (FewRel)& 0.85 (0.04)& \underline{0.86} (0.06)& 0.89 (0.02)& \underline{0.92} (0.02)& 0.85 (0.02)& \underline{0.93} (0.00)\\ \midrule
League (FewRel)& 0.73 (0.01)& \underline{0.82} (0.08)& 0.80 (0.11)& \underline{0.84} (0.14)& 0.80 (0.01)& \underline{0.88} (0.03)\\ \midrule
Platform (FewRel)& 0.71 (0.00)& \underline{0.81} (0.02)& 0.79 (0.02)& \underline{0.88} (0.02)& 0.70 (0.03)& \underline{0.79} (0.10)\\ \midrule
Participating Team (FewRel)& 0.85 (0.02)& \underline{0.94} (0.01)& 0.82 (0.09)& \underline{0.87} (0.12)& 0.78 (0.01)& \underline{0.89} (0.02)\\ \midrule
Military Branch (FewRel)& 0.82 (0.03)& \underline{0.88} (0.02)& 0.83 (0.02)& \underline{0.90} (0.04)& 0.82 (0.03)& \underline{0.92} (0.02)\\ \midrule
Movement (FewRel)& 0.82 (0.00)& \underline{0.91} (0.01)& 0.77 (0.02)& \underline{0.87} (0.02)& 0.79 (0.03)& \underline{0.86} (0.04)\\ \midrule
Sibling (FewRel)& 0.82 (0.02)& \underline{0.91} (0.01)& 0.76 (0.02)& \underline{0.85} (0.04)& 0.81 (0.01)& \underline{0.89} (0.03)\\ \midrule
Successful Candidate (FewRel)& 0.79 (0.01)& \underline{0.87} (0.01)& 0.80 (0.02)& \underline{0.91} (0.02)& 0.88 (0.01)& \underline{0.96} (0.01)\\ \midrule
Taxon Rank (FewRel)& 0.79 (0.05)& \underline{0.88} (0.08)& 0.96 (0.02)& \underline{0.99} (0.00)& 0.81 (0.05)& \underline{0.94} (0.04)\\ \midrule
Tributary (FewRel)& 0.73 (0.00)& \underline{0.85} (0.04)& 0.82 (0.03)& \underline{0.92} (0.04)& 0.89 (0.01)& \underline{0.97} (0.01)\\ \midrule
Occupation (FewRel)& 0.73 (0.01)& \underline{0.78} (0.01)& 0.73 (0.02)& \underline{0.74} (0.06)& 0.54 (0.00)& \underline{0.55} (0.02)\\ \midrule
Winner (FewRel)& 0.75 (0.01)& \underline{0.82} (0.03)& 0.80 (0.02)& \underline{0.84} (0.02)& 0.69 (0.02)& \underline{0.76} (0.03)\\ \midrule
Genre (FewRel)& 0.74 (0.02)& \underline{0.77} (0.01)& 0.72 (0.05)& \underline{0.77} (0.03)& 0.69 (0.04)& \underline{0.73} (0.02)\\
\end{xltabular}
