# Supplementary material for: Embroid: Unsupervised Prediction Smoothing Can Improve Few-Shot Classification
Source: arXiv:2307.11031 source file (2023-07-20)
Supplement: Supplementary file 5 [file closed_models.tex]

\begin{xltabular}{\textwidth}{lll}
\caption{J1-Large Performance on a Subset of Tasks (F1)} \label{tab:j1_large} \\

\multicolumn{1}{l}{\textbf{Task}} & \multicolumn{1}{l}{\name} & \multicolumn{1}{l}{\textbf{Base Prompt}} \\ \toprule 
\endfirsthead

\multicolumn{3}{l}%
{\tablename\ \thetable{} -- continued from previous page} \\
\multicolumn{1}{l}{\textbf{Task}} &  \multicolumn{1}{l}{\name} & \multicolumn{1}{l}{\textbf{Base Prompt}} \\ \toprule
\endhead

%\hline \multicolumn{3}{|r|}{{Continued on next page}} \\ \hline
\endfoot

\bottomrule
\endlastfoot 
dbpedia\_album & \underline{0.99} & 0.94 \\ \midrule 
dbpedia\_company & \underline{0.83} & 0.74 \\ \midrule 
dbpedia\_film & \underline{0.89} & 0.82 \\ \bottomrule 

\end{xltabular}
