# Supplementary material for: Embroid: Unsupervised Prediction Smoothing Can Improve Few-Shot Classification
Source: arXiv:2307.11031 source file (2023-07-20)
Supplement: Supplementary file 6 [file single_prompt_domain_breakdown.tex]

\begin{table}
    \centering
    \begin{tabular}{lSSSSSS}
        \toprule
        \multirow{2}{*}{Domain} &
          \multicolumn{3}{c}{\% of tasks where \name is better} &
          \multicolumn{3}{c}{Average improvement (F1)} \\
          & {G} & {S} & {L} & {G} & {S} & {L}  \\
          \midrule
        GPT-JT-6B-v1 & 0.983 & 0.833 & 0.721 & 0.069 & 0.036 & 0.023\\ \midrule
    bloom-7b1 & 0.796 & 0.737 & 0.750 & 0.035 & 0.019 & 0.025\\ \midrule
    opt-6.7b & 0.879 & 0.500 & 0.762 & 0.066 & 0.004 & 0.023\\ 
    \bottomrule
    \end{tabular}
   \caption{Improvements for \name in the single-prompt setting, disaggregated by domain (i.e. \textbf{G}eneral, \textbf{S}cience, \textbf{L}aw).}
\label{tab:single_prompt_domain_breakdown}
\end{table}
